# Supplementary material for: The Limiting Poisson Law of Massive MIMO Detection with Box Relaxation
Source: arXiv:2006.08416 source file (2020-06-15)
Supplement: Supplementary file 1 [file appendix.tex]

%!TEX root = boxlasso_JSAIT20.tex
\subsection{Properties of Optimization Problem (\ref{eq:tau})}
\label{appen:1Dopt}
In this section, we collect some useful properties of one-dimensional optimization (\ref{eq:tau}), most of which have been studied before in \cite{thrampoulidis2018symbol}.

In general, we consider the following optimization problem parameterized by $t>0$:
\begin{align}
\label{eq:fpstar_t}
f_p(t) &= \min_{\tau>0} F_p(\tau; t, \sampratio) \nonumber \\
&= \min_{\tau>0}\frac{\tau}{2}\left(\sampratio-\frac{1}{2}\right)+\frac{t}{2\tau}+\frac{\tau}{2}\int_{\frac{2}{\tau}}^{\infty}\left(x-\frac{2}{\tau}\right)^{2}Dx.
\end{align}
Note that (\ref{eq:tau}) and the inline optimization of (\ref{eq:Qpstar_theta}) are the cases where $t=\nsdp^2$ and $t=(1+\field)^2\nsdp^2$, respectively. Also we define the square loss function: $R_p(t) \bydef \frac{f_p^2(t)}{2}$ and evidently, $R_p\big[(1+\field)^2\nsdp^2\big] = \optQ(\field)$, where $\optQ(\field)$ is defined in (\ref{eq:Qpstar_theta}).
\subsubsection{Uniqueness of Optimal Solution}
Let $\tau(t)$ be the minimizer of (\ref{eq:fpstar_t}), which is the solution of stationary equation:
\begin{equation}
\underbrace{\sampratio-\frac{1}{2}+\int_{\frac{2}{\tau}}^{\infty}\left(x^{2}-\frac{4}{\tau^{2}}\right)Dx-\frac{t}{\tau^{2}}}_{:=h(\tau)}=0.\label{eq:tau_t_equation}
\end{equation}
By direct differentiation of $h(\tau)$ above, we can show $h'(\tau) = \int_{\frac{2}{\tau}}^{\infty}\frac{8}{\tau^3}Dx+\frac{2t}{\tau^3}>0$, so it is a strictly increasing function. Also $\lim_{\tau\to 0}h(\tau) = -\infty$ and $\lim_{\tau\to\infty}h(\tau) = \sampratio>0$. Therefore, $\tau(t)$ is unique for any $t>0$. Besides, we can directly check that $\tau(t)$ is differentiable with
\begin{equation}\label{eq:tau_deri}
\tau'(t)=\frac{\tau(t)}{8\int_{2/\tau(t)}^{\infty}Dx+2t}>0,
\end{equation}
so $\tau(t)$ is strictly increasing.
\subsubsection{Upper and Lower Bounds of $\tau(t)$}
Since $h\Big(\sqrt{\tfrac{t}{\sampratio}}\Big) < -\frac{1}{2}+\int_{\frac{2}{\tau}}^{\infty}x^{2}Dx<0$, by $h(0^+)<0$, $h(\infty)>0$ and uniqueness of $\tau(t)$, we have $\tau(t)\geq\sqrt{\tfrac{t}{\sampratio}}$. Similarly, we can get $\tau(t)\leq\min\{\sqrt{\tfrac{t}{\sampratio-1/2}},\sqrt{\tfrac{4+t}{\sampratio}}\}$ and $\tau(t)\geq\sqrt{\tfrac{t}{\sampratio-1/2+v_{p}}}
$, where $v_{p} = \int_{b_p}^{\infty}x^{2}Dx$, with $b_p = 2\sqrt{\tfrac{\sampratio-1/2}{t}}$ and evidently, $v_{p}<1/2$. Therefore, $\tau(t)$ can be bounded as:
\begin{equation}\label{eq:tau_t_ublb}
\sqrt{\tfrac{t}{\sampratio-1/2+v_{p}}} \leq \tau(t) \leq \min\Big\{\sqrt{\tfrac{t}{\sampratio-1/2}},\sqrt{\tfrac{4+t}{\sampratio}}\Big\}.
\end{equation}
\subsubsection{Properties of $f_p(t)$}
From (\ref{eq:fpstar_t}) we get $f_p(t)\geq 0$, $f_p'(t)=\frac{1}{2\tau(t)}>0$ and $f_p''(t)=-\frac{\tau'(t)}{2\tau^2(t)}<0$, so $f_p(t)$ is non-negative, strictly increasing and concave. On the other hand, letting $\tau=1$ in (\ref{eq:fpstar_t}) we can get $f_p(t)\leq \frac{t}{2}+C$, where $C$ is a constant.
\subsubsection{Properties of $R_p(t)$}
By chain rule, we have $R_p'(t)=\frac{f_p(t)}{2\tau(t)}$ and $R_p''(t) = \tfrac{\int_{2/\tau(t)}^{\infty}xDx}{\tau(t)(8\int_{2/\tau(t)}^{\infty}Dx+2t)}$. Therefore, $R_p(t)$ is strictly increasing and convex. From (\ref{eq:tau_t_equation}), we can show $R_p'(t)$ is bounded:
\begin{equation}\label{eq:Rpderi_bd}
R_p'(t) = \frac{1}{2}\left[\sampratio-\tfrac{1}{2}+\int_{\frac{2}{\tau(t)}}^{\infty}x^{2}-\tfrac{2x}{\tau(t)}Dx\right]\leq\sampratio.
\end{equation}
On the other hand, $R_p''(t)$ satisfies: $R_p''(t)\leq \frac{\varphi(-2/\tau(t))}{2\tau(t)t}$ and accordingly, $\exists c>0$, s.t.,  $R_p''(t)t\leq \frac{\varphi(-2/\tau(t))}{2\tau(t)}\leq c$. This bound will be used in proving Proposition \ref{prop:Ap_conv}.
\subsection{Proof of Proposition \ref{prop:uniform_convergence}}
\label{appen:uniformconv}
We first prove the pointwise convergence of $g_{p}(v)$ to $\E g_{p}(v)$: there exists $c>0$, s.t., for any $v\in[0,2]$ and $\veps>0$,
\begin{equation}
\P\left(\left|g_{p}(v)-\E g_{p}(v)\right|>\varepsilon\right)\leq ce^{-c^{-1}p\min\left\{ \tfrac{\veps^2}{\sampratio},\veps \right\} }.\label{eq:concentration_Gp_pointwise}
\end{equation}

Recall that $g_{p}(v)=\mathcal{G}_{p}\left( {\vacav}{v} \right)$, so it is equivalent to prove $|\mathcal{{G}}_{p}({\vacav}v)-\E\mathcal{{G}}_{p}({\vacav}v)|\to 0$. We first control the moment generating function of $\mathcal{{G}}_{p}({\vacav}v)-\E\mathcal{{G}}_{p}({\vacav}v)$. Applying Theorem 2.2 of \cite{pisier1986probabilistic}, for $\vb$, which is an i.i.d. copy of $\va$, and $|\lambda|\leq\frac{p}{2\sqrt{2}\pi}$, we have
\begin{align*}
\E[\exp\lambda(\mathcal{{G}}_{p}({\vacav}v)-\E\mathcal{{G}}_{p}({\vacav}v))] &\leq \E e^{ \frac{\pi\lambda}{2}(\vb v)^{\T}\nabla\mathcal{{G}}_{p}({\vacav}v) }\\
&\tleq{\text{(a)}}\E_{\dmtx,\noise}\E_{\vacav}e^{\frac{2\lambda^{2}\pi^{2}}{p}\|\vacav\|^{2}}\\
& =\exp\left[-\frac{n}{2}\log\left(1-\frac{4\lambda^{2}\pi^{2}}{p^{2}}\right)\right]\\
& \tleq{\text{(b)}}\exp\left(\frac{4\sampratio\lambda^{2}\pi^{2}}{p}\right),
\end{align*}
where in step (a), we take expectation over $\vb$ and use $|v|\leq 2$ and $\|\nabla\mathcal{{G}}_{p}({\vacav}v)\| \leq {2\|{\vacav}\|}$, implied by (\ref{eq:Gp_Lipschitz}) and in step (b), we use inequality $\log(1+x)\geq\frac{x}{1+x}$,
for $x>-1$ and the condition $|\lambda|\leq\frac{p}{2\sqrt{2}\pi}$.
As a result, for any $\veps \geq 0$ and $\lambda\in\left[0,\frac{p}{2\sqrt{2}\pi}\right]$,
\begin{align}
\label{eq:Chernoff1}
\P\left( g_{p}(v)-\E g_{p}(v) > \varepsilon \right) & \leq e^{-\lambda\varepsilon+\frac{4\sampratio\lambda^{2}\pi^{2}}{p}}.
\end{align}
After minimizing the exponent on the RHS of (\ref{eq:Chernoff1})
over $\lambda\in\left[0,\frac{p}{2\sqrt{2}\pi}\right]$,
%we get
%\begin{equation}
%\P\left(\mathcal{\widetilde{G}}_{p}(\tilde{\vacav})-\E\mathcal{\widetilde{G}}_{p}(\tilde{\vacav})>\varepsilon\right)\leq e^{-\tfrac{p\varepsilon^{2}}{16\alpha_{p}\pi^{2}}}
%\end{equation}
%and
%similarly for the other direction.
%Hence,
we can get for any $\veps\in[0,\sqrt{8}\pi\sampratio]$, $\P\left(g_{p}(v)-\E g_{p}(v)>\varepsilon\right)\leq e^{-\tfrac{p\varepsilon^{2}}{16\sampratio\pi^{2}}}$; for any $\veps > \sqrt{8}\pi\sampratio$, $\P\left(g_{p}(v)-\E g_{p}(v)>\varepsilon\right)\leq e^{-\tfrac{p\varepsilon}{4\sqrt{2}\pi}}$. The other direction also holds by the same reasoning, so summarizing
\begin{align}
\label{eq:gpv_concentrate}
\P\left(\left|g_{p}(v)-\E g_{p}(v)\right|>\varepsilon\right) &\leq 2 e^{-\tfrac{p}{4\pi}\min\{\tfrac{\veps^2}{4\sampratio \pi}, \tfrac{\veps}{\sqrt{2}}\}}\nonumber\\
&\leq 2 e^{-\tfrac{p}{16\pi^2}\min\{\tfrac{\veps^2}{\sampratio }, \veps\}}.
\end{align}

To show uniform convergence (\ref{eq:concentration_gp_uniform}), it suffices to prove the Lipschitz continuity of $g_{p}(v)$ and $\E g_{p}(v)$. From Lemma 1 of \cite{laurent2000adaptive}, we have for all $x>0$, $\P\Big(\|\vacav\|^2\geq \sampratio +\tfrac{2\sqrt{\sampratio x}}{\sqrt{p}}+\tfrac{2x}{p}\Big)\leq \exp(-x)$.
For any $K\geq2 \sampratio$, letting $x=\left(\tfrac{\sqrt{2}-1}{2}\right)^2pK$, we can get $\P(\|\vacav\|^2-\sampratio\geq K/2)\leq \exp(-\tfrac{pK}{32})$. Therefore, we get for any $K\geq2 \sampratio$,
\begin{align}
\label{eq:K_concentrate}
\P(\|\vacav\|^{2}>K) \leq \P(\|\vacav\|^{2}-\sampratio>K/2) \leq \exp(-\tfrac{pK}{32}).
\end{align}
Combine it with (\ref{eq:gp_derivative_upperbd}), we know for $K\geq2 \sampratio$, $g_{p}(v)$ is $2K$-Lipschitz
with probability greater than $1-\exp(-\tfrac{pK}{32})$.
From (\ref{eq:gp_derivative_upperbd}), we can also get $\left|\frac{d\E g_{p}(v)}{dv}\right|\leq4 \sampratio$, so $\E g_{p}(v)$
is $4 \sampratio$-Lipschitz continuous over $v\in[0,2]$. Combining the Lipschitz continuity
of $g_{p}(v)$ and $\E g_{p}(v)$ with (\ref{eq:concentration_Gp_pointwise}),
we can obtain (\ref{eq:concentration_gp_uniform}) by a standard epsilon-net argument as follows. We discuss over different values of $\veps$:
\begin{enumerate}
  \item If $\veps \geq \sampratio$, we construct an epsilon-net of $[0,2]$ formed by the following points: $v_k = \frac{k}{8}$, $k=1,2,\ldots,16$. For any $v\in[0,2]$, denote $v^{*}$ as the closest point to $v$ in the above epsilon-net. By construction, $|v-v^{*}|\leq \frac{1}{8}$. Suppose $g_{p}(v)$ is $2K$-Lipschitz, then for any $v\in[0,2]$,
      \begin{align}
      |g_{p}(v)-\E g_{p}(v)| &\leq |g_{p}(v)-g_{p}(v^{*})| + |g_{p}(v^{*})-\E g_{p}(v^{*})| + |\E g_{p}(v^{*})-\E g_{p}(v)|\nonumber\\
      &\leq \frac{K}{4} + |g_{p}(v^{*})-\E g_{p}(v^{*})| + \frac{\veps}{2},
      \end{align}
      where we have used Lipschitz continuity of $g_{p}(v)$ and $\E g_{p}(v)$, as well as $\veps \geq \sampratio$. Then $\sup_{v\in[0,2]}|g_{p}(v)-\E g_{p}(v)|\geq 2\veps$, only if at least one of following holds: (i) $K\geq 2\veps\geq 2\sampratio$, (ii) there exists a $k\in[16]$, s.t., $|g_{p}(v_{k})-\E g_{p}(v_{k})| \geq \veps$. Combining (\ref{eq:gpv_concentrate}) and (\ref{eq:K_concentrate}) and applying the union bound, we get for $\veps\geq \sampratio$,
      \begin{equation}
      \label{eq:gpv_concentrate1}
       \P(\sup_{v\in[0,2]}|g_{p}(v)-\E g_{p}(v)|\geq 2\veps)\leq 18 e^{-\tfrac{p\veps}{16\pi^2} }.
      \end{equation}
  \item If $\sqrt{\frac{\sampratio}{p}}\leq\veps\leq \sampratio$, we construct an epsilon-net of $[0,2]$ formed by the following points: $v_k = 2k/\lceil\frac{16\sampratio}{\veps}\rceil$, $k=1,2,\ldots,\lceil\frac{16\sampratio}{\veps}\rceil$. In this case, for any $v\in[0,2]$, we have $|v-v^{*}|\leq \frac{\veps}{8\sampratio}$. Then similar as previous argument, we have $\sup_{v\in[0,2]}|g_{p}(v)-\E g_{p}(v)|\geq 2\veps$, only if at least one of following holds: (i) $g_{p}(v)$ is not $4\sampratio$-Lipschitz, (ii) there exists a $k \leq \lceil\frac{16\sampratio}{\veps}\rceil$, s.t., $|g_{p}(v_{k})-\E g_{p}(v_{k})| \geq \veps$. Combining (\ref{eq:gpv_concentrate}) and (\ref{eq:K_concentrate}) and applying the union bound, we get for $\sqrt{\frac{\sampratio}{p}}\leq\veps\leq \sampratio$,
      \begin{equation}
      \label{eq:gpv_concentrate2}
       \P(\sup_{v\in[0,2]}|g_{p}(v)-\E g_{p}(v)|\geq 2\veps)\leq \frac{32\sampratio}{\veps} e^{-\tfrac{p\veps^2}{16\pi^2\sampratio} }.
      \end{equation}
  \item If $\veps \leq \sqrt{\frac{\sampratio}{p}}$, then the RHS of (\ref{eq:gpv_concentrate2}) is greater than $1$, so it holds trivially.
\end{enumerate}
Combining (\ref{eq:gpv_concentrate1}) and (\ref{eq:gpv_concentrate2}), we get for any $\veps > 0$,
\begin{equation}
\label{eq:gpv_concentrate3}
\P(\sup_{v\in[0,2]}|g_{p}(v)-\E g_{p}(v)|\geq \veps)\leq \frac{32\sampratio}{\veps} e^{-\tfrac{p}{64\pi^2}\min\{\tfrac{\veps^2}{\sampratio }, \veps\}},
\end{equation}
which directly implies (\ref{eq:concentration_gp_uniform}).
\subsection{Approximate $k$-wise Independence }
\label{appen:ApproximateIndependence}
\subsubsection{$\big\{ \va_{i}^{\T}\vu_{\backslash i}^{*}\big\} _{i\in[k]} \tapprox{d} \big\{ \va_{i}^{\T}\vu_{\backslash[k]}^{*}\big\} _{i\in[k]}$}
We first prove joint distribution of $\big\{ \va_{i}^{\T}\vu_{\backslash i}^{*}\big\} _{i\in[k]}$
is closed to $\big\{ \va_{i}^{\T}\vu_{\backslash[k]}^{*}\big\} _{i\in[k]}$. To prove this, we can show $\va_{i}^{\T}\vu_{\backslash i}^{*}\approx \va_{i}^{\T}\vu_{\backslash [k]}^{*}$, $\forall i\in[k]$ and use the fact that $\{\vu_{\backslash i}^{*}\}_{i\in[k]}$ and $\vu_{\backslash [k]}^{*}$ are in the same probability space.
%An elementary step
%is to show the difference between $\va_{i}^{\T}\vu_{\backslash[i]}^{*}$
%and $\va_{i}^{\T}\vu_{\backslash[i+1]}^{*}$ is small with high probability, which is following lemma.
\begin{lem}
\label{lem:a1t_deltaUn1_concentrate}$\exists C,c>0$, s.t., $\forall\veps>0$
and $i=1,2,\ldots,p-1$,
\begin{equation}
\P\left(\left|\va_{i}^{\T}(\vu_{\backslash[i]}^{*}-\vu_{\backslash[i+1]}^{*})\right|>\varepsilon\right)\leq ce^{-c^{-1} p\min\left\{ \veps^{2},\veps\right\}}.\label{eq:a1t_deltaUn1_concentrate}
\end{equation}
\end{lem}
\begin{IEEEproof}
To lighten notation, define $\Delta_{[i]}\bydef\vu_{\backslash[i]}^{*}-\vu_{\backslash[i+1]}^{*}$.
Similar as (\ref{eq:ux_Lipschitz}), we can get $\|\Delta_{[i]}\|\leq2\|\va_{i+1}\|$.
Therefore, $\exists C,c>0$, s.t., $\forall\veps>0$ and $D>0$,
Therefore, $\exists C,c>0$, s.t., $\forall\veps>0$ and $D>0$,
\begin{align*}
\P\left(|\va_{i}^{\T}\Delta_{[i]}|>\varepsilon\right) & \leq \P\left(|\va_{i}^{\T}\Delta_{[i]}|>\varepsilon\bigcap\|\Delta_{[i]}\|\leq D\right)+\P\left(\|\Delta_{[i]}\|>D\right)\\
 & \leq\P\left(\left|\va_{i}^{\T}\tfrac{D\Delta_{[i]}}{\|\Delta_{[i]}\|}\right|>\veps\right)+\P\left(\|\va_{i+1}\|>\tfrac{D}{2}\right)\\
 & \leq e^{-\tfrac{p\veps^{2}}{2D^{2}}}+Ce^{-C^{-1}p\left(\tfrac{D}{2\sqrt{\sampratio}}-1\right)_{+}^{2}},
\end{align*}
where $(x)_{+}\bydef \max\{x,0\}$. Then by choosing a fixed $D$ for small $\veps$ and $D \asymp \sqrt{\veps}$ for large $\veps$, we can get (\ref{eq:a1t_deltaUn1_concentrate}).
\end{IEEEproof}
\begin{lem}
\label{lem:leave1_leavek_compare}, $\exists c>0$, s.t., $\forall b_{i}\in\R$,
$i=1,2,\ldots,k$ and $\veps>0$,
\begin{equation}
\P\left(\bigcap_{i=1}^{k}\left\{ \va_{i}^{\T}\vu_{\backslash i}^{*}\leq b_{i}\right\} \right)\geq\P\left(\bigcap_{i=1}^{k}\left\{ \va_{i}^{\T}\vu_{\backslash[k]}^{*}\leq b_{i}-\veps\right\} \right)-ck^{2}e^{-c^{-1}p\min\left\{ \tfrac{\veps^{2}}{k^{2}},\tfrac{\veps}{k}\right\} }\label{eq:leave1_leavek_compare_1}
\end{equation}
and
\begin{equation}
\P\left(\bigcap_{i=1}^{k}\left\{ \va_{i}^{\T}\vu_{\backslash i}^{*}\leq b_{i}\right\} \right)\leq\P\left(\bigcap_{i=1}^{k}\left\{ \va_{i}^{\T}\vu_{\backslash[k]}^{*}\leq b_{i}+\veps\right\} \right)+ck^{2}e^{-c^{-1}p\min\left\{ \tfrac{\veps^{2}}{k^{2}},\tfrac{\veps}{k}\right\} }.\label{eq:leave1_leavek_compare_2}
\end{equation}
\end{lem}
\begin{IEEEproof}
From Lemma \ref{lem:a1t_deltaUn1_concentrate}, $\forall k\in[p]$,
$\exists c>0$, s.t., $\forall\veps>0$,
\begin{align*}
\P\left(\left|\va_{1}^{\T}(\vu_{\backslash1}^{*}-\vu_{\backslash[k]}^{*})\right|>\veps\right) & \leq\sum_{i=1}^{k-1}\P\left(\left|\va_{1}^{\T}(\vu_{\backslash[i]}^{*}-\vu_{\backslash[i+1]}^{*})\right|>\tfrac{\veps}{k-1}\right)\\
 & \leq cke^{-c^{-1}p\min\left\{ \tfrac{\veps^{2}}{k^{2}},\tfrac{\veps}{k}\right\} }.
\end{align*}
By exchangeability of $\left\{ \va_{i}^{\T}\vu_{\backslash i}^{*},\va_{i}^{\T}\vu_{\backslash[k]}^{*}\right\} _{i\in[k]}$,
we have $\forall i\in[k]$, it holds that
\[
\P\left(\left|\va_{i}^{\T}(\vu_{\backslash i}^{*}-\vu_{\backslash[k]}^{*})\right|>\veps\right)\leq cke^{-c^{-1}p\min\left\{ \tfrac{\veps^{2}}{k^{2}},\tfrac{\veps}{k}\right\} }.
\]
Therefore, we have $\forall \veps>0$,
\begin{align*}
 \P\left(\bigcap_{i=1}^{k}\{\va_{i}^{\T}\vu_{\backslash i}^{*}\leq b_{i}\}\right)
&=  \P\left(\bigcap_{i=1}^{k}\{\va_{i}^{\T}\vu_{\backslash[k]}^{*}\leq b_{i}-\va_{i}^{\T}(\vu_{\backslash i}^{*}-\vu_{\backslash[k]}^{*})\}\right)\\
&\leq \P\left(\bigcap_{i=1}^{k}\{\va_{i}^{\T}\vu_{\backslash[k]}^{*}\leq b_{i}+\veps\}\right)+\P\left(\bigcup_{i=1}^{k}\{\left|\va_{i}^{\T}(\vu_{\backslash i}^{*}-\vu_{\backslash[k]}^{*})\right|>\veps\}\right)\\
&\leq \P\left(\bigcap_{i=1}^{k}\{\va_{i}^{\T}\vu_{\backslash[k]}^{*}\leq b_{i}+\veps\}\right)+ck^{2}e^{-c^{-1}p\min\left\{ \tfrac{\veps^{2}}{k^{2}},\tfrac{\veps}{k}\right\} },
\end{align*}
which is (\ref{eq:leave1_leavek_compare_1}). The other direction (\ref{eq:leave1_leavek_compare_2}) can be obtained in the same way.
\end{IEEEproof}
\subsubsection{$\big\{ \va_{i}^{\T}\vu_{\backslash[k]}^{*}\big\} _{i\in[k]} \tapprox{d} \big\{ \va_{i}^{\T}\widetilde{\vu}_{\backslash[k]}^{*}\big\} _{i\in[k]}$}
Next we show the joint distribution of $\big\{ \va_{i}^{\T}\vu_{\backslash[k]}^{*}\big\} _{i\in[k]}$
is closed to $\big\{ \va_{i}^{\T}\widetilde{\vu}_{\backslash[k]}^{*}\big\} _{i\in[k]}$. First we show $\tfrac{\|\vu_{\backslash[k]}^{*}\|}{\sqrt{p}}\approx\tfrac{\|\widetilde{\vu}_{\backslash[k]}^{*}\|}{\sqrt{p}}=\optS$.
\begin{lem}
\label{lem:concentration_unotk_norm}When $k\leq\tfrac{p}{2}$, $\exists C,c>0$,
s.t. $\forall\veps>0$,
\begin{equation}
\P\left(\left|\tfrac{\|\vu_{\backslash[k]}^{*}\|}{\sqrt{p}}-\optS\right|>\veps\right)\leq ce^{-c^{-1}p\left(\veps-\tfrac{Ck}{p}\right)_{+}^{2}}.\label{eq:concentration_unotk_norm}
\end{equation}
\end{lem}
\begin{IEEEproof}
By definition of $\vu_{\backslash[k]}^{*}$, we can get
\begin{align}
\tfrac{\|\vu_{\backslash[k]}^{*}\|}{\sqrt{p}} &= \tfrac{1}{\sqrt{p}} \min_{\vx\in[-1,1]^{p-k}}\|{\dmtx}_{\backslash[k]}\vx-({\dmtx}_{\backslash[k]}\vbeta_{\backslash[k]}+{\vw})\|\nonumber\\
&= \frac{\sampratio}{\delta_{p,\backslash[k]}}\cdot\frac{\min_{\vx\in[-1,1]^{p-k}}\|\widetilde{\dmtx}_{\backslash[k]}\vx-(\widetilde{\dmtx}_{\backslash[k]}\vbeta_{\backslash[k]}+\widetilde{\vw})\|}{\sqrt{p-k}},
\end{align}
where $\delta_{p,\backslash[k]}=\tfrac{n}{p-k}$, i.e., the
sampling ratio after removing $k$ predictors, $\widetilde{\dmtx}_{\backslash[k]}\iid\mathcal{N}\big(0,\tfrac{1}{p-k}\big)$
and $\widetilde{\vw}\sim\mathcal{N}\Big(\boldsymbol{0},\tfrac{\delta_{p,\backslash[k]} \nsdp^{2}}{\sampratio}\mI_{n}\Big)$. Define
\begin{align}
S_{p}^{*}(\delta) & \bydef\tfrac{\sampratio}{\delta}\min_{\tau>0}F_{p}\left(\tau;\tfrac{\delta\nsdp^{2}}{\sampratio},\delta\right),\label{eq:Spstar_alpha}
\end{align}
where $F_{p}$ is defined in (\ref{eq:F}). Similar to Lemma \ref{lem:Qp_theta_concentration}, we
can get for $k\leq\tfrac{p}{2}$, $\exists c>0$, s.t., $\forall\veps>0$,
\begin{equation}
\P\left(\left|\tfrac{\|\vu_{\backslash[k]}^{*}\|}{\sqrt{p}}-S_{p,\backslash[k]}^{*}\right|>\veps\right)\leq ce^{-(p-k)\veps^{2}/c},\label{eq:equiv_notk_conv}
\end{equation}
where $S_{p,\backslash[k]}^{*}\bydef S_{p}^{*}(\delta_{p,\backslash[k]})$.

On the other hand, $|S_{p,\backslash[k]}^{*} - \optS|$ can be bounded
as follows. From (\ref{eq:Spstar_alpha}),
we can show $\exists C>0$, s.t., $\left|\tfrac{dS_{p}^{*}(\delta)}{d\delta}\right|\leq C$.
Since $\optS = S_{p}^{*}(\sampratio)$ and $S_{p,\backslash[k]}^{*} = S_{p}^{*}(\delta_{p,\backslash[k]})$,
by mean value theorem, we can get for $k\leq\tfrac{p}{2}$, $\exists C>0$, s.t.,
\begin{equation}
\left|S_{p,\backslash[k]}^{*} - \optS \right|\leq\tfrac{Ck}{p}.\label{eq:Sp_notk_Qpstar_diff}
\end{equation}
Now we combine (\ref{eq:equiv_notk_conv})
and (\ref{eq:Sp_notk_Qpstar_diff}). If $\veps-\tfrac{Ck}{p}>0$,
\begin{align*}
\P\left(\left|\tfrac{\|\vu_{\backslash[k]}^{*}\|}{\sqrt{p}}-\optS\right|>\veps\right)
 & \leq ce^{-c^{-1}p\left(\veps-\tfrac{Ck}{p}\right)^{2}}
\end{align*}
and if $\veps-\tfrac{Ck}{p}\leq0$, we can choose $c\geq1$ and (\ref{eq:concentration_unotk_norm})
trivially holds.
\end{IEEEproof}
Based on Lemma \ref{lem:concentration_unotk_norm}, we can now show
$\va_{i}^{\T}\vu_{\backslash[k]}^{*}\approx \va_{i}^{\T}\widetilde{\vu}_{\backslash[k]}^{*}$,
if $k$ is not too large.
\begin{lem}
\label{lem:aiT_ustardiff_bd} If $k\leq\sqrt{p}$, then $\exists c>0$,
s.t., for any $\veps>0$,
\begin{equation}
\P\left(\left|\va_{i}^{\T}(\vu_{\backslash[k]}^{*}-\widetilde{\vu}_{\backslash[k]}^{*})\right|>\veps\right)\leq ce^{-\sqrt{p}\veps/c}.\label{eq:aiT_ustardiff_bd}
\end{equation}
\end{lem}
\begin{IEEEproof}
The proof is similar to Lemma \ref{lem:a1t_deltaUn1_concentrate} and is omitted here.
\end{IEEEproof}
Using Lemma \ref{lem:aiT_ustardiff_bd}, we can show joint distributions
of $\left\{ \va_{i}^{\T}\vu_{\backslash[k]}^{*}\right\} _{i\in[k]}$
and $\left\{ \va_{i}^{\T}\widetilde{\vu}_{\backslash[k]}^{*}\right\} _{i\in[k]}$ are similar.
\begin{lem}
\label{lem:leavek_leaveknormalized_compare}If $k\leq\sqrt{p}$, $\exists c>0$,
s.t., $\forall b_{i}\in\R$, $i=1,2,\ldots,p$ and $\veps>0$,
\begin{align}
\P(\va_{i}^{\T}\vu_{\backslash[k]}^{*}\leq b_{i},i\in[k])\leq & \P\left(\va_{i}^{\T}\widetilde{\vu}_{\backslash[k]}^{*}\leq b_{i}+\veps,i\in[k]\right)+cke^{-\sqrt{p}\veps/c}\label{eq:leavek_leaveknormalized_compare_1}
\end{align}
and
\begin{align}
\P(\va_{i}^{\T}\vu_{\backslash[k]}^{*}\leq b_{i},i\in[k])\geq & \P\left(\va_{i}^{\T}\widetilde{\vu}_{\backslash[k]}^{*}\leq b_{i}-\veps,i\in[k]\right)-cke^{-\sqrt{p}\veps/c}.\label{eq:leavek_leaveknormalized_compare_2}
\end{align}
\end{lem}
\begin{IEEEproof}
The proof is similar to Lemma \ref{lem:leave1_leavek_compare} and is omitted here.
\end{IEEEproof}
\subsubsection{Proof of Proposition \ref{prop:approx_indep_Gaussian}}
The proof follows directly Lemma \ref{lem:leave1_leavek_compare} and \ref{lem:leavek_leaveknormalized_compare}.
\subsubsection{Proof of Proposition \ref{prop:joint_k_Bern_approx_indep_1}}
Letting $b_{i}=-A_{p}^{*}$ in (\ref{eq:joint_k_approx_indep_Gaussian}), we have
\begin{align}
\P\Big(\bigcap_{i=1}^{k}\left\{ \tilde{\sgli}_{i}\neq\beta_{i}\right\} \Big)
 & \geq \Phi^{k}\left(-\tfrac{1+\veps/A_{p}^{*}}{\opttau}\right)-\widetilde{\Delta}_{p,k}\label{eq:joint_k_approx_indep_Gaussian_4_0}\\
 & \geq \Phi^{k}\left(-\tfrac{1}{\opttau}\right)\left[1-\tfrac{h({1}/{\opttau})\veps}{\opttau A_{p}^{*}}\right]^{k}-\widetilde{\Delta}_{p,k},\label{eq:joint_k_approx_indep_Gaussian_4_1}
\end{align}
where $h(x)=\frac{\varphi(-x)}{\Phi(-x)}$ is the so-called inverse Mills ratio.  By (\ref{eq:Apstar_bd}), (\ref{eq:joint_k_approx_indep_Gaussian_4_1}) and (\ref{eq:inverse_mills_ratio_bd}) given in Appendix \ref{appen:mills}, if $\sigma_{p}\geq\frac{1}{\log p}$, then $\exists c>0$, s.t., $\forall k\leq\sqrt{p}$ and small enough $\veps>0$,
\begin{align}
\P\Big(\bigcap_{i=1}^{k}\left\{ \tilde{\sgli}_{i}\neq\beta_{i}\right\} \Big) & \tgeq{\text{}}\Phi^{k}\left(-\tfrac{1}{\opttau}\right)\Big(1-\tfrac{ck\veps}{\sigma_{p}^{2}}\Big)-\widetilde{\Delta}_{p,k}.\label{eq:joint_k_approx_indep_Gaussian_4}
\end{align}
On the other hand, we can also get the similar bounds as (\ref{eq:joint_k_approx_indep_Gaussian_4_0}) and (\ref{eq:joint_k_approx_indep_Gaussian_4}) for the other direction.

Now consider the case $k\leq p^{\tfrac{1}{8}}$. Accordingly, we set
$\veps=p^{-\tfrac{1}{4}}$. Then $\exists c>0$,
s.t.,
\begin{equation}
\widetilde{\Delta}_{p,k}\leq cp^{1/4}e^{-\sqrt[4]{p}/c}.\label{eq:tilde_Delta_pk_order}
\end{equation}
As a result, from (\ref{eq:Apstar_bd}), (\ref{eq:joint_k_approx_indep_Gaussian_4_0}) and (\ref{eq:tilde_Delta_pk_order}), if $k\leq p^{\tfrac{1}{8}}$,
$\exists c>0$, s.t.,
\begin{equation}
\P\Big(\bigcap_{i=1}^{k}\left\{ \tilde{\sgli}_{i}\neq\beta_{i}\right\} \Big)\geq \Phi^{k}\Big(-\tfrac{1+cp^{-\tfrac{1}{4}}}{\opttau}\Big)-ce^{-\sqrt[4]{p}/c}.\label{eq:joint_k_Bern_approx_indep1}
\end{equation}
Meanwhile, we can also get
\begin{align}
\P\Big(\bigcap_{i=1}^{k}\left\{ \tilde{\sgli}_{i}\neq\beta_{i}\right\} \Big)-\Phi^{k}\left(-\tfrac{1}{\opttau}\right) & \geq -c\left[\Phi^{k}\left(-\tfrac{1}{\opttau}\right)kp^{-\tfrac{1}{4}}L_{p}+p^{1/4}e^{-p^{\tfrac{1}{4}}/c}\right]\nonumber \\
 & \geq -\Phi^{k}\left(-\tfrac{1}{\opttau}\right)kp^{-\tfrac{1}{4}}L_{p}.\label{eq:joint_k_Bern_approx_indep_3}
\end{align}
The other directions of (\ref{eq:joint_k_Bern_approx_indep1}) and (\ref{eq:joint_k_Bern_approx_indep_3}) can be derived in the same way, which lead to (\ref{eq:joint_k_Bern_approx_indep_2}) and (\ref{eq:joint_k_Bern_approx_indep_1}).
%%%%%%%%%%%%%% details of the other direction %%%%%%%%%%%%%%%%%%%%%%%%%%%%%%%%%%%%%%%%%%%%%%%%%
%
%Similarly, for the other direction, for any $k\leq\sqrt{p}$ and $\veps>0$,
%\begin{align}
%\P\left(\bigcap_{i=1}^{k}\left\{ \tilde{\sgli}_{i}\neq\beta_{i}\right\} \right) & \leq\Phi^{k}\left(-\tfrac{1-\veps/A_{p}^{*}}{\opttau}\right)+\widetilde{\Delta}_{p,k}\label{eq:joint_k_approx_indep_Gaussian_3_0}
%\end{align}
%Also $\exists c>0$, s.t., for $\sigma_{p}\geq\frac{1}{\log p}$
%and small enough $\veps>0$,
%\begin{align}
%\P\left(\bigcap_{i=1}^{k}\left\{ \tilde{\sgli}_{i}\neq\beta_{i}\right\} \right) & \leq\Phi^{k}\left(-\tfrac{1}{\opttau}\right)\left(1+\tfrac{ck\veps}{\sigma_{p}^{2}}\right)+\widetilde{\Delta}_{p,k}.\label{eq:joint_k_approx_indep_Gaussian_3}
%\end{align}
%
%%%%%%%%%%%%%%%%%%%%%%%%%%%%%%%%%%%%%%%%%%%%%%%%%%%%%%%%%
\subsection{Properties of Gaussian Tail}
\label{appen:mills}
Here we gather some results about tail probability of standard Gaussian that will be used in our proof. Let $\Phi(x)$ and $\varphi(x)$ be the CDF and PDF of standard Gaussian distribution. A well known result is: for $x>0$,
\begin{equation}
\frac{1}{x}-\frac{1}{x^{3}} \leq m(x) \leq\frac{1}{x},\label{eq:mills_ratio}
\end{equation}
where $m(x) \bydef \frac{\Phi(-x)}{\varphi(-x)}$ for $x>0$, is known as Mills ratio. Correspondingly, the inverse Mills ratio is defined as $h(x)\bydef1/m(x)$. This provides us a way to approximate tail probability $\Phi(-x)$ by $\varphi(x)$, which has an explicit form. In view of (\ref{eq:tau_t_ublb}) and (\ref{eq:mills_ratio}), $\exists M>1$,
s.t., $\forall\epsilon\in[-1/2,1/2]$,
\begin{equation}
\tfrac{1+\epsilon}{\opttau}\leq h\Big(-\tfrac{1+\epsilon}{\opttau}\Big) \leq\tfrac{M(1+\epsilon)}{\opttau}.\label{eq:inverse_mills_ratio_bd}
\end{equation}
Meanwhile, from (\ref{eq:inverse_mills_ratio_bd}), $\forall\epsilon\in[-1/2,1/2]$,
\begin{align}
\Phi\left(-\tfrac{1+\epsilon}{\opttau}\right) & \leq\tfrac{1}{1+\epsilon}\sqrt{\tfrac{\nsdp^{2}}{\sampratio-1/2}}e^{-\frac{(1+\epsilon)^{2}(\sampratio-1/2)}{2\nsdp^{2}}}\label{eq:Phi_1_tau_upbd}
\end{align}
and
\begin{align}
\Phi\left(-\tfrac{1+\epsilon}{\opttau}\right) & \geq\tfrac{1}{M(1+\epsilon)}\sqrt{\tfrac{\nsdp^{2}}{\sampratio}}e^{-\frac{(1+\epsilon)^{2}(\sampratio-1/2+v_{p})}{2\nsdp^{2}}},\label{eq:Phi_1_tau_lowerbd}
\end{align}
where $v_{p} = \int_{b_p}^{\infty}x^{2}Dx$, with $b_p = 2\sqrt{\tfrac{\sampratio-1/2}{t}}$.
%\subsection{Limiting Poisson Law of $\tneb$}
\subsection{Proof of Proposition \ref{prop:Poisson_convergence}}
\label{appen:tneb_proof}
%\subsubsection{Proof of Proposition \ref{prop:pt_tildeNEB}}

%\subsubsection{Proof of Proposition \ref{prop:Poisson_convergence}}
If $\ptline \geq2$, from (\ref{eq:E_tildeNe_ubd}) and (\ref{eq:Phi_1_tau_upbd}),
we know $\exists c>0$, s.t., $\lambda_{p}\leq cp^{-\tfrac{1}{2}}$
and $\E\tneb\leq cp^{-\tfrac{1}{2}}$. Hence, $d_{\text{TV}}(\tneb,\mathscr{P}_{\optlam})$ can be bounded
as:
\begin{align*}
d_{\text{TV}}(\tneb,\mathscr{P}_{\optlam}) & =\frac{1}{2}\sum_{k=0}^{\infty}\left|\P\left(\tneb=k\right)-\frac{\optlam^{k}}{k!}e^{-\optlam}\right|\\
 & \leq\frac{1}{2}\left|\P\left(\tneb=0\right)-e^{-\optlam}\right|+\frac{1}{2}\P\left(\tneb\geq1\right)+\frac{1}{2}\left(1-e^{-\optlam}\right)\\
 & \leq2cp^{-\tfrac{1}{2}}.
\end{align*}
On the other hand, if $\ptline<2$,
then for large enough $p$, it holds that $\sigma_{p}\geq\frac{1}{\log p}$.
Choose $L$ in (\ref{eq:Bonferroni_1}) to be $L=\left\lfloor 5\log p\right\rfloor .$
Without loss of generality, assume $L-k$ is odd (otherwise we add
$L$ by $1$). Then from Bonferroni's inequality (\ref{eq:Bonferroni_1}), for $k\leq\left\lfloor \log p\right\rfloor $,
\begin{align}
\P\left(\tneb=k\right) & \leq\sum_{m=k}^{L-1}\binom{m}{k}(-1)^{m-k}S_{m}\nonumber \\
 & \leq\sum_{m=0}^{L-1-k}\frac{(-1)^{m}}{k!m!}p^{m+k}S_{[m+k]}\nonumber \\
 & \tleq{\text{(a)}}\sum_{m=0}^{L-1-k}\frac{(-1)^{m}}{k!m!}p^{m+k}\Phi^{m+k}\left(-\tfrac{1}{\opttau}\right)\left(1+p^{-1/4}L_{p}\right)\nonumber \\
 & \tleq{\text{(b)}}\frac{\lambda_{p}^{k}}{k!}e^{-\lambda_{p}}\left(1+\frac{\lambda_{p}^{L-k}e^{\lambda_{p}}}{(L-k)!}\right)\left(1+p^{-1/4}L_{p}\right)\nonumber \\
 & \tleq{\text{(c)}}\frac{\lambda_{p}^{k}}{k!}e^{-\lambda_{p}}\left(1+\left(\frac{\lambda_{p}e}{L-k}\right)^{L-k}e^{\lambda_{p}-1}\right)\left(1+p^{-1/4}L_{p}\right)\nonumber \\
 & \tleq{\text{(d)}}\frac{\lambda_{p}^{k}}{k!}e^{-\lambda_{p}}\left(1+(e^{5}/4^{4})^{\log p}\right)\left(1+p^{-1/4}L_{p}\right),\label{eq:P_k_upper_bd}
\end{align}
where step (a) follows from (\ref{eq:joint_k_Bern_approx_indep_1}),
step (b) follows from Taylor approximation of $e^{x}$ with Lagrange
remainder and the fact that $L-k$ is odd, in step (c) we use inequality
$n!\geq e\left(\tfrac{n}{e}\right)^{n}$ and step (d) follows from conditions $L=\left\lfloor 5\log p\right\rfloor$, $k\leq\left\lfloor \log p\right\rfloor$ and $\optlam\leq\log p$. In a similar manner, for the other direction, we can also obtain
\begin{align}
\P\left(\tneb=k\right) & \geq\frac{\lambda_{p}^{k}}{k!}e^{-\lambda_{p}}\left(1-(e^{5}/4^{4})^{\log p}\right)\left(1-p^{-1/4}L_{p}\right).\label{eq:P_k_lower_bd}
\end{align}
For large enough $p$, by (\ref{eq:P_k_upper_bd}), (\ref{eq:P_k_lower_bd})
and $\lambda_{p}\leq \log p$,
\begin{equation}
\left|\P\left(\tneb=k\right)-\frac{\lambda_{p}^{k}}{k!}e^{-\lambda_{p}}\right|\leq\frac{\lambda_{p}^{k}}{k!}e^{-\lambda_{p}}p^{-1/4}L_{p}.\label{eq:P_k_bd_1}
\end{equation}
Then $d_{\text{TV}}(\tneb,\mathscr{P}_{\lambda_{p}})$
can be bounded as
\begin{align*}
d_{\text{TV}}(\tneb,\mathscr{P}_{\lambda_{p}}) & =\frac{1}{2}\sum_{k=0}^{\infty}\left|\P\left(\tneb=k\right)-\frac{\lambda_{p}^{k}}{k!}e^{-\lambda_{p}}\right|\\
 & \leq\frac{1}{2}\sum_{k=0}^{L}\left|\P\left(\tneb=k\right)-\frac{\lambda_{p}^{k}}{k!}e^{-\lambda_{p}}\right|+\frac{1}{2}\sum_{k=L+1}^{\infty}\P\left(\tneb=k\right)+\frac{1}{2}\sum_{k=L+1}^{\infty}\frac{\lambda_{p}^{k}}{k!}e^{-\lambda_{p}}\\
 & \tleq{\text{(a)}}\frac{p^{-1/4}L_{p}}{2}\sum_{k=0}^{L}\frac{\lambda_{p}^{k}}{k!}e^{-\lambda_{p}}+\frac{1}{2}\left[1-\sum_{k=0}^{L}\frac{\lambda_{p}^{k}}{k!}e^{-\lambda_{p}}\left(1-p^{-1/4}L_{p}\right)\right]+\frac{1}{2}\sum_{k=L+1}^{\infty}\frac{\lambda_{p}^{k}}{k!}e^{-\lambda_{p}}\\
 & \tleq{\text{(b)}}p^{-1/4}L_{p}+e^{\lambda_{p}}\left(\frac{e\lambda_{p}}{L}\right)^{L}\\
 & \tleq{\text{(c)}}p^{-1/4}L_{p},
\end{align*}
where in step (a) we use (\ref{eq:P_k_bd_1}), in step (b) we use
Chernoff's bound for tail probability of Poisson random variable and
in step (c) we use the condition $L=\left\lfloor 5\log p\right\rfloor $
and $\lambda_{p}\leq\log p$.
